# Supplementary material for: The nuclear and integrated far-infrared emission of nearby Seyfert galaxies
Source: arXiv:1603.04235 ancillary file (2016-03-14)
Supplement: Supplementary file 1 [file Observing_programs_table.pdf]

**Table 1.** *Herschel*/PACS and SPIRE observing programs.

| Galaxy       | Observation ID | Instrument | Wavelengths ( $\mu\text{m}$ ) | PI                |
|--------------|----------------|------------|-------------------------------|-------------------|
| ESO 323-G077 | 1342236922     | PACS       | 70, 160                       | Mushotzky R.      |
| ESO 323-G077 | 1342236923     | PACS       | 70, 160                       | Mushotzky R.      |
| ESO 323-G077 | 1342236202     | SPIRE      | 250, 350, 500                 | Mushotzky R.      |
| IC 5063      | 1342216469     | PACS       | 70, 160                       | Sánchez-Portal M. |
| IC 5063      | 1342216470     | PACS       | 70, 160                       | Sánchez-Portal M. |
| IC 5063      | 1342216471     | PACS       | 100, 160                      | Sánchez-Portal M. |
| IC 5063      | 1342216472     | PACS       | 100, 160                      | Sánchez-Portal M. |
| IC 5063      | 1342206208     | SPIRE      | 250, 350, 500                 | Sánchez-Portal M. |
| Mrk 1066     | 1342249288     | PACS       | 70, 160                       | Alonso-Herrero A. |
| Mrk 1066     | 1342249289     | PACS       | 70, 160                       | Alonso-Herrero A. |
| Mrk 1066     | 1342249286     | PACS       | 100, 160                      | Alonso-Herrero A. |
| Mrk 1066     | 1342249287     | PACS       | 100, 160                      | Alonso-Herrero A. |
| Mrk 1066     | 1342239823     | SPIRE      | 250, 350, 500                 | Alonso-Herrero A. |
| NGC 1068     | 1342189194     | PACS       | 70, 160                       | Wilson C.         |
| NGC 1068     | 1342189195     | PACS       | 70, 160                       | Wilson C.         |
| NGC 1068     | 1342189425     | SPIRE      | 250, 350, 500                 | Wilson C.         |
| NGC 1320     | 1342249144     | PACS       | 70, 160                       | Alonso-Herrero A. |
| NGC 1320     | 1342249145     | PACS       | 70, 160                       | Alonso-Herrero A. |
| NGC 1320     | 1342249146     | PACS       | 100, 160                      | Alonso-Herrero A. |
| NGC 1320     | 1342249147     | PACS       | 100, 160                      | Alonso-Herrero A. |
| NGC 1320     | 1342239845     | SPIRE      | 250, 350, 500                 | Alonso-Herrero A. |
| NGC 1365     | 1342183550     | PACS       | 70, 160                       | Calibration       |
| NGC 1365     | 1342183551     | PACS       | 70, 160                       | Calibration       |
| NGC 1365     | 1342183552     | PACS       | 100, 160                      | Calibration       |
| NGC 1365     | 1342183553     | PACS       | 100, 160                      | Calibration       |
| NGC 1365     | 1342201436     | SPIRE      | 250, 350, 500                 | Sánchez-Portal M. |
| NGC 1386     | 1342216452     | PACS       | 70, 160                       | Sánchez-Portal M. |
| NGC 1386     | 1342216453     | PACS       | 70, 160                       | Sánchez-Portal M. |
| NGC 1386     | 1342216454     | PACS       | 100, 160                      | Sánchez-Portal M. |
| NGC 1386     | 1342216455     | PACS       | 100, 160                      | Sánchez-Portal M. |
| NGC 1386     | 1342214554     | SPIRE      | 250, 350, 500                 | Sánchez-Portal M. |
| NGC 1808     | 1342204260     | PACS       | 70, 160                       | Sturm E.          |
| NGC 1808     | 1342204261     | PACS       | 70, 160                       | Sturm E.          |
| NGC 1808     | 1342204262     | PACS       | 100, 160                      | Sturm E.          |
| NGC 1808     | 1342204263     | PACS       | 100, 160                      | Sturm E.          |
| NGC 1808     | 1342203633     | SPIRE      | 250, 350, 500                 | Sturm E.          |
| NGC 2110     | 1342242542     | PACS       | 70, 160                       | Mushotzky R.      |
| NGC 2110     | 1342242543     | PACS       | 70, 160                       | Mushotzky R.      |
| NGC 2110     | 1342252037     | PACS       | 100, 160                      | Mushotzky R.      |
| NGC 2110     | 1342252038     | PACS       | 100, 160                      | Mushotzky R.      |
| NGC 2110     | 1342227709     | SPIRE      | 250, 350, 500                 | Mushotzky R.      |
| NGC 2273     | 1342243812     | PACS       | 70, 160                       | Alonso-Herrero A. |
| NGC 2273     | 1342243813     | PACS       | 70, 160                       | Alonso-Herrero A. |
| NGC 2273     | 1342243814     | PACS       | 100, 160                      | Alonso-Herrero A. |
| NGC 2273     | 1342243815     | PACS       | 100, 160                      | Alonso-Herrero A. |
| NGC 2273     | 1342240032     | SPIRE      | 250, 350, 500                 | Alonso-Herrero A. |
| NGC 2992     | 1342221109     | PACS       | 70, 160                       | Sánchez-Portal M. |
| NGC 2992     | 1342221110     | PACS       | 70, 160                       | Sánchez-Portal M. |
| NGC 2992     | 1342221111     | PACS       | 100, 160                      | Sánchez-Portal M. |
| NGC 2992     | 1342221112     | PACS       | 100, 160                      | Sánchez-Portal M. |
| NGC 2992     | 1342198866     | SPIRE      | 250, 350, 500                 | Sánchez-Portal M. |
| NGC 3081     | 1342210628     | PACS       | 70, 160                       | Sánchez-Portal M. |
| NGC 3081     | 1342210629     | PACS       | 70, 160                       | Sánchez-Portal M. |
| NGC 3081     | 1342210630     | PACS       | 100, 160                      | Sánchez-Portal M. |
| NGC 3081     | 1342210631     | PACS       | 100, 160                      | Sánchez-Portal M. |
| NGC 3081     | 1342210523     | SPIRE      | 250, 350, 500                 | Sánchez-Portal M. |
| NGC 3227     | 1342221146     | PACS       | 70, 160                       | Spinoglio L.      |
| NGC 3227     | 1342221147     | PACS       | 70, 160                       | Spinoglio L.      |
| NGC 3227     | 1342255954*    | PACS       | 100, 160                      | Alonso-Herrero A. |
| NGC 3227     | 1342255955*    | PACS       | 100, 160                      | Alonso-Herrero A. |
| NGC 3227     | 1342197318     | SPIRE      | 250, 350, 500                 | Eales S.          |

Notes.— The Observation ID marked with an asterisk indicates that this observation is used for the mosaic of 160  $\mu\text{m}$  but not for the 100  $\mu\text{m}$ .

Table 1 – *continued*

| Galaxy   | Observation ID | Instrument | Wavelengths ( $\mu\text{m}$ ) | PI                |
|----------|----------------|------------|-------------------------------|-------------------|
| NGC 3281 | 1342221845     | PACS       | 70, 160                       | Sánchez-Portal M. |
| NGC 3281 | 1342221846     | PACS       | 70, 160                       | Sánchez-Portal M. |
| NGC 3281 | 1342221847     | PACS       | 100, 160                      | Sánchez-Portal M. |
| NGC 3281 | 1342221848     | PACS       | 100, 160                      | Sánchez-Portal M. |
| NGC 3281 | 1342201483     | SPIRE      | 250, 350, 500                 | Sánchez-Portal M. |
| NGC 3783 | 1342222503     | PACS       | 70, 160                       | Sánchez-Portal M. |
| NGC 3783 | 1342222504     | PACS       | 70, 160                       | Sánchez-Portal M. |
| NGC 3783 | 1342222505     | PACS       | 100, 160                      | Sánchez-Portal M. |
| NGC 3783 | 1342222506     | PACS       | 100, 160                      | Sánchez-Portal M. |
| NGC 3783 | 1342202198     | SPIRE      | 250, 350, 500                 | Sánchez-Portal M. |
| NGC 4051 | 1342221164     | PACS       | 70, 160                       | Spinoglio L.      |
| NGC 4051 | 1342221165     | PACS       | 70, 160                       | Spinoglio L.      |
| NGC 4051 | 1342256164*    | PACS       | 100, 160                      | Alonso-Herrero A. |
| NGC 4051 | 1342256165*    | PACS       | 100, 160                      | Alonso-Herrero A. |
| NGC 4051 | 1342210502     | SPIRE      | 250, 350, 500                 | Spinoglio L.      |
| NGC 4151 | 1342188217     | PACS       | 70, 160                       | Wilson C.         |
| NGC 4151 | 1342188218     | PACS       | 70, 160                       | Wilson C.         |
| NGC 4151 | 1342255503*    | PACS       | 100, 160                      | Alonso-Herrero A. |
| NGC 4151 | 1342255504*    | PACS       | 100, 160                      | Alonso-Herrero A. |
| NGC 4151 | 1342188588     | SPIRE      | 250, 350, 500                 | Wilson C.         |
| NGC 4253 | 1342235128     | PACS       | 70, 160                       | Mushotzky R.      |
| NGC 4253 | 1342235129     | PACS       | 70, 160                       | Mushotzky R.      |
| NGC 4253 | 1342248046     | PACS       | 100, 160                      | Alonso-Herrero A. |
| NGC 4253 | 1342248047     | PACS       | 100, 160                      | Alonso-Herrero A. |
| NGC 4253 | 1342234910     | SPIRE      | 250, 350, 500                 | Mushotzky R.      |
| NGC 4258 | 1342220105     | PACS       | 70, 160                       | Sánchez-Portal M. |
| NGC 4258 | 1342220106     | PACS       | 70, 160                       | Sánchez-Portal M. |
| NGC 4258 | 1342220108     | PACS       | 70, 160                       | Sánchez-Portal M. |
| NGC 4258 | 1342220107     | PACS       | 100, 160                      | Sánchez-Portal M. |
| NGC 4258 | 1342201364     | SPIRE      | 250, 350, 500                 | Sánchez-Portal M. |
| NGC 4258 | 1342222664     | SPIRE      | 250, 350, 500                 | Mushotzky R.      |
| NGC 4388 | 1342233038     | PACS       | 70, 160                       | Davies J.         |
| NGC 4388 | 1342233039     | PACS       | 70, 160                       | Davies J.         |
| NGC 4388 | 1342248482     | SPIRE      | 250, 350, 500                 | Alonso-Herrero A. |
| NGC 4507 | 1342237736     | PACS       | 70, 160                       | Mushotzky R.      |
| NGC 4507 | 1342237737     | PACS       | 70, 160                       | Mushotzky R.      |
| NGC 4507 | 1342234818     | SPIRE      | 250, 350, 500                 | Mushotzky R.      |
| NGC 4579 | 1342212664     | PACS       | 70, 160                       | Kennicutt R.      |
| NGC 4579 | 1342212666     | PACS       | 70, 160                       | Kennicutt R.      |
| NGC 4579 | 1342212665     | PACS       | 100, 160                      | Kennicutt R.      |
| NGC 4579 | 1342212667     | PACS       | 100, 160                      | Kennicutt R.      |
| NGC 4579 | 1342188795     | SPIRE      | 250, 350, 500                 | Eales S.          |
| NGC 4594 | 1342213103     | PACS       | 70, 160                       | Kennicutt R.      |
| NGC 4594 | 1342213105     | PACS       | 70, 160                       | Kennicutt R.      |
| NGC 4594 | 1342213104     | PACS       | 100, 160                      | Kennicutt R.      |
| NGC 4594 | 1342213106     | PACS       | 100, 160                      | Kennicutt R.      |
| NGC 4594 | 1342188815     | SPIRE      | 250, 350, 500                 | Kennicutt R.      |
| NGC 4725 | 1342198481     | PACS       | 70, 160                       | Kennicutt R.      |
| NGC 4725 | 1342198483     | PACS       | 70, 160                       | Kennicutt R.      |
| NGC 4725 | 1342198482     | PACS       | 100, 160                      | Kennicutt R.      |
| NGC 4725 | 1342198484     | PACS       | 100, 160                      | Kennicutt R.      |
| NGC 4725 | 1342188763     | SPIRE      | 250, 350, 500                 | Eales S.          |
| NGC 5135 | 1342237916     | PACS       | 70, 160                       | Sanders D.        |
| NGC 5135 | 1342237917     | PACS       | 70, 160                       | Sanders D.        |
| NGC 5135 | 1342237918     | PACS       | 100, 160                      | Sanders D.        |
| NGC 5135 | 1342237919     | PACS       | 100, 160                      | Sanders D.        |
| NGC 5135 | 1342202248     | SPIRE      | 250, 350, 500                 | Van der Werf P.   |
| NGC 5347 | 1342246878     | PACS       | 70, 160                       | Alonso-Herrero A. |
| NGC 5347 | 1342246879     | PACS       | 70, 160                       | Alonso-Herrero A. |
| NGC 5347 | 1342246880     | PACS       | 100, 160                      | Alonso-Herrero A. |
| NGC 5347 | 1342246881     | PACS       | 100, 160                      | Alonso-Herrero A. |
| NGC 5347 | 1342259455     | SPIRE      | 250, 350, 500                 | Alonso-Herrero A. |

Table 1 – *continued*

| Galaxy   | Observation ID | Instrument | Wavelengths ( $\mu\text{m}$ ) | PI                |
|----------|----------------|------------|-------------------------------|-------------------|
| NGC 5506 | 1342223830     | PACS       | 70, 160                       | Sánchez-Portal M. |
| NGC 5506 | 1342223831     | PACS       | 70, 160                       | Sánchez-Portal M. |
| NGC 5506 | 1342223832     | PACS       | 100, 160                      | Sánchez-Portal M. |
| NGC 5506 | 1342223833     | PACS       | 100, 160                      | Sánchez-Portal M. |
| NGC 5506 | 1342213466     | SPIRE      | 250, 350, 500                 | Sánchez-Portal M. |
| NGC 7130 | 1342218550     | PACS       | 70, 160                       | Spinoglio L.      |
| NGC 7130 | 1342218551     | PACS       | 70, 160                       | Spinoglio L.      |
| NGC 7130 | 1342210527     | SPIRE      | 250, 350, 500                 | Spinoglio L.      |
| NGC 7172 | 1342220760     | PACS       | 70, 160                       | Spinoglio L.      |
| NGC 7172 | 1342220761     | PACS       | 70, 160                       | Spinoglio L.      |
| NGC 7172 | 1342209301     | SPIRE      | 250, 350, 500                 | Spinoglio L.      |
| NGC 7213 | 1342232480     | PACS       | 70, 160                       | Mushotzky R.      |
| NGC 7213 | 1342232481     | PACS       | 70, 160                       | Mushotzky R.      |
| NGC 7213 | 1342244160     | SPIRE      | 250, 350, 500                 | Mushotzky R.      |
| NGC 7465 | 1342237360     | PACS       | 70, 160                       | Mushotzky R.      |
| NGC 7465 | 1342237361     | PACS       | 70, 160                       | Mushotzky R.      |
| NGC 7465 | 1342237445     | PACS       | 100, 160                      | Alonso-Herrero A. |
| NGC 7465 | 1342237446     | PACS       | 100, 160                      | Alonso-Herrero A. |
| NGC 7465 | 1342258533     | PACS       | 100, 160                      | Crocker A.        |
| NGC 7465 | 1342258534     | PACS       | 100, 160                      | Crocker A.        |
| NGC 7465 | 1342234763     | SPIRE      | 250, 350, 500                 | Mushotzky R.      |
| NGC 7465 | 1342259379     | SPIRE      | 250, 350, 500                 | Crocker A.        |
| NGC 7479 | 1342237358     | PACS       | 70, 160                       | Mushotzky R.      |
| NGC 7479 | 1342237359     | PACS       | 70, 160                       | Mushotzky R.      |
| NGC 7479 | 1342237443     | PACS       | 100, 160                      | Alonso-Herrero A. |
| NGC 7479 | 1342237444     | PACS       | 100, 160                      | Alonso-Herrero A. |
| NGC 7479 | 1342234760     | SPIRE      | 250, 350, 500                 | Mushotzky R.      |
| NGC 7582 | 1342221132     | PACS       | 70, 160                       | Spinoglio L.      |
| NGC 7582 | 1342221133     | PACS       | 70, 160                       | Spinoglio L.      |
| NGC 7582 | 1342245180*    | PACS       | 100, 160                      | Alonso-Herrero A. |
| NGC 7582 | 1342245181*    | PACS       | 100, 160                      | Alonso-Herrero A. |
| NGC 7582 | 1342210529     | SPIRE      | 250, 350, 500                 | Spinoglio L.      |
