# Supplementary material for: The nuclear and integrated far-infrared emission of nearby Seyfert galaxies
Source: arXiv:1603.04235 ancillary file (2016-03-14)
Supplement: Supplementary file 2 [file Photometry_tables.pdf]

**Table 1.** Aperture photometry for  $r = 1$  kpc.

| Galaxy       | radius<br>(arcsec) | Flux<br>$70\mu\text{m}$ (Jy) | Flux<br>$100\mu\text{m}$ (Jy) | Flux<br>$160\mu\text{m}$ (Jy) | Flux<br>$250\mu\text{m}$ (Jy) | Flux<br>$350\mu\text{m}$ (Jy) | Flux<br>$500\mu\text{m}$ (Jy) |
|--------------|--------------------|------------------------------|-------------------------------|-------------------------------|-------------------------------|-------------------------------|-------------------------------|
| ESO 323-G077 | 3.43               |                              |                               |                               |                               |                               |                               |
| IC 5063      | 4.13               |                              |                               |                               |                               |                               |                               |
| Mrk 1066     | 4.21               | 12 $\pm$ 1                   |                               |                               |                               |                               |                               |
| NGC 1068     | 14.32              | 164 $\pm$ 16                 |                               | 88 $\pm$ 9                    | 28 $\pm$ 3                    |                               |                               |
| NGC 1320     | 5.81               | 1.8 $\pm$ 0.2                | 2.0 $\pm$ 0.2                 |                               |                               |                               |                               |
| NGC 1365     | 9.59               | 63 $\pm$ 6                   | 81 $\pm$ 8                    | 87 $\pm$ 9                    |                               |                               |                               |
| NGC 1386     | 19.46              | 6.9 $\pm$ 0.7                | 9.2 $\pm$ 0.9                 | 7.6 $\pm$ 0.8                 | 3.0 $\pm$ 0.3                 | 1.1 $\pm$ 0.1                 |                               |
| NGC 1808     | 16.80              | 107 $\pm$ 11                 | 121 $\pm$ 12                  | 102 $\pm$ 10                  | 33 $\pm$ 3                    |                               |                               |
| NGC 2110     | 6.37               | 4.6 $\pm$ 0.5                | 5.2 $\pm$ 0.5                 |                               |                               |                               |                               |
| NGC 2273     | 7.19               | 7.0 $\pm$ 0.7                | 7.9 $\pm$ 0.8                 |                               |                               |                               |                               |
| NGC 2992     | 6.05               | 7.1 $\pm$ 0.7                | 8.5 $\pm$ 0.9                 |                               |                               |                               |                               |
| NGC 3081     | 6.03               | 2.2 $\pm$ 0.2                | 2.4 $\pm$ 0.2                 |                               |                               |                               |                               |
| NGC 3227     | 10.01              | 8.3 $\pm$ 0.8                |                               | 8.5 $\pm$ 0.9                 |                               |                               |                               |
| NGC 3281     | 4.61               | 7.0 $\pm$ 0.7                | 6.9 $\pm$ 0.7                 |                               |                               |                               |                               |
| NGC 3783     | 5.71               | 1.8 $\pm$ 0.2                | 1.4 $\pm$ 0.1                 |                               |                               |                               |                               |
| NGC 4051     | 15.99              | 3.5 $\pm$ 0.4                |                               | 4.1 $\pm$ 0.4                 | 1.3 $\pm$ 0.1                 |                               |                               |
| NGC 4151     | 10.16              | 4.9 $\pm$ 0.5                |                               | 2.0 $\pm$ 0.2                 |                               |                               |                               |
| NGC 4253     | 3.36               |                              |                               |                               |                               |                               |                               |
| NGC 4258     | 25.85              | 6.5 $\pm$ 0.6                | 12 $\pm$ 1                    | 12 $\pm$ 1                    | 5.2 $\pm$ 0.5                 | 2.0 $\pm$ 0.2                 |                               |
| NGC 4388     | 12.13              | 6.8 $\pm$ 0.7                |                               | 7.1 $\pm$ 0.7                 |                               |                               |                               |
| NGC 4507     | 3.46               |                              |                               |                               |                               |                               |                               |
| NGC 4579     | 12.13              | 2.7 $\pm$ 0.3                | 3.8 $\pm$ 0.4                 | 2.2 $\pm$ 0.2                 |                               |                               |                               |
| NGC 4594     | 16.24              | 1.2 $\pm$ 0.1                | 1.7 $\pm$ 0.2                 | 1.7 $\pm$ 0.2                 | 1.0 $\pm$ 0.1                 |                               |                               |
| NGC 4725     | 7.64               | 0.23 $\pm$ 0.02              | 0.34 $\pm$ 0.03               |                               |                               |                               |                               |
| NGC 5135     | 3.57               |                              |                               |                               |                               |                               |                               |
| NGC 5347     | 5.13               | 1.1 $\pm$ 0.1                | 1.2 $\pm$ 0.1                 |                               |                               |                               |                               |
| NGC 5506     | 6.88               | 8.8 $\pm$ 0.9                | 8.3 $\pm$ 0.8                 |                               |                               |                               |                               |
| NGC 7130     | 3.00               |                              |                               |                               |                               |                               |                               |
| NGC 7172     | 5.49               | 5.8 $\pm$ 0.6                |                               |                               |                               |                               |                               |
| NGC 7213     | 8.28               | 1.4 $\pm$ 0.1                |                               |                               |                               |                               |                               |
| NGC 7465     | 7.26               | 3.7 $\pm$ 0.4                | 4.5 $\pm$ 0.5                 |                               |                               |                               |                               |
| NGC 7479     | 6.37               |                              | 10 $\pm$ 1                    |                               |                               |                               |                               |
| NGC 7582     | 9.38               | 57 $\pm$ 6                   |                               | 44 $\pm$ 4                    |                               |                               |                               |

**Table 2.** Aperture photometry for  $r = 2$  kpc.

| Galaxy       | radius<br>(arcsec) | Flux<br>70 $\mu$ m (Jy) | Flux<br>100 $\mu$ m (Jy) | Flux<br>160 $\mu$ m (Jy) | Flux<br>250 $\mu$ m (Jy) | Flux<br>350 $\mu$ m (Jy) | Flux<br>500 $\mu$ m (Jy) |
|--------------|--------------------|-------------------------|--------------------------|--------------------------|--------------------------|--------------------------|--------------------------|
| ESO 323-G077 | 6.85               | 6.9 $\pm$ 0.7           |                          |                          |                          |                          |                          |
| IC 5063      | 8.27               | 4.5 $\pm$ 0.5           | 3.6 $\pm$ 0.4            |                          |                          |                          |                          |
| Mrk 1066     | 8.42               | 12 $\pm$ 1              | 12 $\pm$ 1               |                          |                          |                          |                          |
| NGC 1068     | 28.65              | 253 $\pm$ 25            |                          | 186 $\pm$ 19             | 65 $\pm$ 7               | 23 $\pm$ 2               | 8.0 $\pm$ 0.8            |
| NGC 1320     | 11.62              | 2.2 $\pm$ 0.2           | 2.8 $\pm$ 0.3            | 2.3 $\pm$ 0.2            |                          |                          |                          |
| NGC 1365     | 19.19              | 96 $\pm$ 10             | 131 $\pm$ 13             | 128 $\pm$ 13             | 49 $\pm$ 5               | 19 $\pm$ 2               |                          |
| NGC 1386     | 38.92              | 7.1 $\pm$ 0.7           | 10 $\pm$ 1               | 8.8 $\pm$ 0.9            | 3.7 $\pm$ 0.4            | 1.5 $\pm$ 0.1            | 0.50 $\pm$ 0.05          |
| NGC 1808     | 33.54              | 119 $\pm$ 12            | 142 $\pm$ 14             | 118 $\pm$ 12             | 42 $\pm$ 4               | 16 $\pm$ 2               | 3.4 $\pm$ 0.3            |
| NGC 2110     | 12.73              | 5.1 $\pm$ 0.5           | 6.2 $\pm$ 0.6            | 4.5 $\pm$ 0.5            |                          |                          |                          |
| NGC 2273     | 14.37              | 7.3 $\pm$ 0.7           | 8.8 $\pm$ 0.9            | 6.4 $\pm$ 0.6            | 2.3 $\pm$ 0.2            |                          |                          |
| NGC 2992     | 12.10              | 8.8 $\pm$ 0.9           | 11 $\pm$ 1               | 8.9 $\pm$ 0.9            |                          |                          |                          |
| NGC 3081     | 12.06              | 2.5 $\pm$ 0.3           | 2.9 $\pm$ 0.3            | 2.3 $\pm$ 0.2            |                          |                          |                          |
| NGC 3227     | 20.03              | 9.1 $\pm$ 0.9           |                          | 11 $\pm$ 1               | 4.4 $\pm$ 0.4            | 1.7 $\pm$ 0.2            |                          |
| NGC 3281     | 9.23               | 7.3 $\pm$ 0.7           | 7.5 $\pm$ 0.8            | 5.0 $\pm$ 0.5            |                          |                          |                          |
| NGC 3783     | 11.43              | 2.0 $\pm$ 0.2           | 1.9 $\pm$ 0.2            | 1.0 $\pm$ 0.1            |                          |                          |                          |
| NGC 4051     | 31.98              | 4.4 $\pm$ 0.5           |                          | 6.6 $\pm$ 0.7            | 3.0 $\pm$ 0.3            | 1.2 $\pm$ 0.1            | 0.41 $\pm$ 0.04          |
| NGC 4151     | 20.32              | 5.7 $\pm$ 0.6           |                          | 3.2 $\pm$ 0.3            | 0.80 $\pm$ 0.08          | 0.26 $\pm$ 0.03          |                          |
| NGC 4253     | 6.73               | 4.2 $\pm$ 0.4           | 4.2 $\pm$ 0.4            |                          |                          |                          |                          |
| NGC 4258     | 51.70              | 14 $\pm$ 1              | 27 $\pm$ 3               | 29 $\pm$ 3               | 13 $\pm$ 1               | 5.3 $\pm$ 0.5            | 1.8 $\pm$ 0.2            |
| NGC 4388     | 24.27              | 9 $\pm$ 1               |                          | 12 $\pm$ 1               | 13.8 $\pm$ 0.4           | 1.4 $\pm$ 0.1            |                          |
| NGC 4507     | 6.92               | 3.7 $\pm$ 0.4           |                          |                          |                          |                          |                          |
| NGC 4579     | 24.27              | 3.4 $\pm$ 0.4           | 5.7 $\pm$ 0.6            | 4.4 $\pm$ 0.4            | 1.8 $\pm$ 0.2            | 0.69 $\pm$ 0.07          |                          |
| NGC 4594     | 32.48              | 2.3 $\pm$ 0.3           | 4.4 $\pm$ 0.4            | 5.2 $\pm$ 0.5            | 2.9 $\pm$ 0.3            | 1.5 $\pm$ 0.2            | 0.74 $\pm$ 0.07          |
| NGC 4725     | 15.28              | 0.59 $\pm$ 0.06         | 1.0 $\pm$ 0.1            | 1.0 $\pm$ 0.1            | 0.43 $\pm$ 0.04          |                          |                          |
| NGC 5135     | 7.15               | 20 $\pm$ 2              | 27 $\pm$ 3               |                          |                          |                          |                          |
| NGC 5347     | 10.26              | 1.2 $\pm$ 0.1           | 1.4 $\pm$ 0.1            | 1.2 $\pm$ 0.1            |                          |                          |                          |
| NGC 5506     | 13.75              | 9.0 $\pm$ 0.9           | 8.8 $\pm$ 0.9            | 5.7 $\pm$ 0.6            | 1.9 $\pm$ 0.2            |                          |                          |
| NGC 7130     | 6.00               | 16 $\pm$ 2              |                          |                          |                          |                          |                          |
| NGC 7172     | 10.97              | 7.3 $\pm$ 0.7           |                          | 10 $\pm$ 1               |                          |                          |                          |
| NGC 7213     | 16.57              | 2.1 $\pm$ 0.2           |                          | 1.0 $\pm$ 0.1            | 0.92 $\pm$ 0.09          |                          |                          |
| NGC 7465     | 14.53              | 4.4 $\pm$ 0.4           | 5.7 $\pm$ 0.6            | 4.4 $\pm$ 0.4            | 1.5 $\pm$ 0.2            |                          |                          |
| NGC 7479     | 12.73              | 10 $\pm$ 1              | 11 $\pm$ 1               | 8.5 $\pm$ 0.9            |                          |                          |                          |
| NGC 7582     | 18.75              | 60 $\pm$ 6              |                          | 51 $\pm$ 5               | 18 $\pm$ 2               |                          |                          |

**Table 3.** Integrated photometry

| Galaxy       | radius<br>(arcsec) | Flux<br>70 $\mu$ m (Jy) | Flux<br>100 $\mu$ m (Jy) | Flux<br>160 $\mu$ m (Jy) | Flux<br>250 $\mu$ m (Jy) | Flux<br>350 $\mu$ m (Jy) | Flux<br>500 $\mu$ m (Jy) |
|--------------|--------------------|-------------------------|--------------------------|--------------------------|--------------------------|--------------------------|--------------------------|
| ESO 323-G077 | 50                 | 6.8 $\pm$ 0.8           |                          | 7.1 $\pm$ 0.8            | 3.2 $\pm$ 0.3            | 1.3 $\pm$ 0.1            | 0.43 $\pm$ 0.04          |
| IC 5063      | 60                 | 4.7 $\pm$ 0.5           | 4.6 $\pm$ 0.5            | 3.7 $\pm$ 0.4            | 2.1 $\pm$ 0.2            | 0.9 $\pm$ 0.1            | 0.30 $\pm$ 0.04          |
| Mrk 1066     | 50                 | 12 $\pm$ 1              | 13 $\pm$ 1               | 8.5 $\pm$ 0.9            | 3.0 $\pm$ 0.3            | 1.1 $\pm$ 0.1            | 0.33 $\pm$ 0.04          |
| NGC 1068     | 230                | 292 $\pm$ 30            |                          | 299 $\pm$ 30             | 117 $\pm$ 12             | 45 $\pm$ 5               | 15 $\pm$ 2               |
| NGC 1320     | 50                 | 2.4 $\pm$ 0.3           | 3.4 $\pm$ 0.4            | 3.0 $\pm$ 0.4            | 1.5 $\pm$ 0.2            | 0.58 $\pm$ 0.07          | 0.20 $\pm$ 0.03          |
| NGC 1365     | 365                | 143 $\pm$ 16            | 216 $\pm$ 23             | 220 $\pm$ 23             | 102 $\pm$ 10             | 44 $\pm$ 5               | 16 $\pm$ 2               |
| NGC 1386     | 60                 | 7.0 $\pm$ 0.7           | 10 $\pm$ 1               | 8.9 $\pm$ 0.9            | 3.9 $\pm$ 0.4            | 1.6 $\pm$ 0.2            | 0.57 $\pm$ 0.06          |
| NGC 1808     | 250                | 134 $\pm$ 14            | 173 $\pm$ 18             | 153 $\pm$ 16             | 62 $\pm$ 7               | 24 $\pm$ 3               | 8 $\pm$ 1                |
| NGC 2110     | 50                 | 5.2 $\pm$ 0.6           | 6.8 $\pm$ 0.7            | 5.2 $\pm$ 0.6            | 2.0 $\pm$ 0.2            | 0.79 $\pm$ 0.09          | 0.25 $\pm$ 0.03          |
| NGC 2273     | 50                 | 7.4 $\pm$ 0.8           | 10 $\pm$ 1               | 7.5 $\pm$ 0.8            | 3.3 $\pm$ 0.3            | 1.3 $\pm$ 0.1            | 0.48 $\pm$ 0.05          |
| NGC 2992     | 80                 | 10 $\pm$ 1              | 13 $\pm$ 1               | 11 $\pm$ 1               | 4.8 $\pm$ 0.5            | 2.0 $\pm$ 0.2            | 0.76 $\pm$ 0.09          |
| NGC 3081     | 60                 | 3.0 $\pm$ 0.4           | 4.1 $\pm$ 0.6            | 4.6 $\pm$ 0.5            | 2.3 $\pm$ 0.2            | 0.90 $\pm$ 0.09          | 0.31 $\pm$ 0.04          |
| NGC 3227     | 110                | 12 $\pm$ 1              |                          | 21 $\pm$ 2               | 12 $\pm$ 1               | 5.2 $\pm$ 0.6            | 1.8 $\pm$ 0.2            |
| NGC 3281     | 120                | 7.4 $\pm$ 0.9           | 8 $\pm$ 1                | 7.1 $\pm$ 0.8            | 2.8 $\pm$ 0.4            | 1.1 $\pm$ 0.2            | 0.30 $\pm$ 0.09          |
| NGC 3783     | 50                 | 3.5 $\pm$ 0.4           | 5.2 $\pm$ 0.6            | 5.1 $\pm$ 0.6            | 2.5 $\pm$ 0.3            | 1.0 $\pm$ 0.1            | 0.36 $\pm$ 0.04          |
| NGC 4051     | 170                | 15 $\pm$ 4              |                          | 31 $\pm$ 4               | 22 $\pm$ 2               | 10 $\pm$ 1               | 3.9 $\pm$ 0.4            |
| NGC 4151     | 150                | 8 $\pm$ 1               |                          | 9 $\pm$ 1                | 4.3 $\pm$ 0.6            | 1.9 $\pm$ 0.3            | 0.6 $\pm$ 0.2            |
| NGC 4253     | 40                 | 4.2 $\pm$ 0.5           | 4.5 $\pm$ 0.5            | 3.0 $\pm$ 0.3            | 1.2 $\pm$ 0.1            | 0.45 $\pm$ 0.05          | 0.10 $\pm$ 0.01          |
| NGC 4258     | 290                | 39 $\pm$ 5              | 72 $\pm$ 10              | 101 $\pm$ 11             | 58 $\pm$ 7               | 27 $\pm$ 5               | 10 $\pm$ 1               |
| NGC 4388     | 130                | 13 $\pm$ 2              |                          | 20 $\pm$ 2               | 8.1 $\pm$ 0.8            | 3.3 $\pm$ 0.4            | 1.2 $\pm$ 0.2            |
| NGC 4507     | 50                 | 5.0 $\pm$ 0.6           |                          | 5.8 $\pm$ 0.7            | 2.5 $\pm$ 0.3            | 1.0 $\pm$ 0.1            | 0.32 $\pm$ 0.04          |
| NGC 4579     | 200                | 11 $\pm$ 3              | 26 $\pm$ 5               | 35 $\pm$ 4               | 20 $\pm$ 2               | 9 $\pm$ 1                | 3.1 $\pm$ 0.5            |
| NGC 4594     | 280                | 9 $\pm$ 2               | 27 $\pm$ 7               | 38 $\pm$ 5               | 24 $\pm$ 3               | 11 $\pm$ 1               | 4.3 $\pm$ 0.7            |
| NGC 4725     | 450                | 10 $\pm$ 4              | 28 $\pm$ 7               | 45 $\pm$ 5               | 33 $\pm$ 4               | 17 $\pm$ 2               | 7 $\pm$ 1                |
| NGC 5135     | 80                 | 22 $\pm$ 2              | 33 $\pm$ 3               | 29 $\pm$ 3               | 13 $\pm$ 1               | 5.3 $\pm$ 0.5            | 1.7 $\pm$ 0.2            |
| NGC 5347     | 60                 | 1.7 $\pm$ 0.3           | 2.6 $\pm$ 0.3            | 3.2 $\pm$ 0.4            | 1.8 $\pm$ 0.2            | 0.84 $\pm$ 0.09          | 0.30 $\pm$ 0.04          |
| NGC 5506     | 70                 | 8.9 $\pm$ 0.9           | 9 $\pm$ 1                | 7.4 $\pm$ 0.8            | 3.0 $\pm$ 0.3            | 1.2 $\pm$ 0.1            | 0.39 $\pm$ 0.04          |
| NGC 7130     | 60                 | 20 $\pm$ 2              |                          | 22 $\pm$ 2               | 9.2 $\pm$ 0.9            | 3.6 $\pm$ 0.4            | 1.1 $\pm$ 0.1            |
| NGC 7172     | 60                 | 7.6 $\pm$ 0.9           |                          | 14 $\pm$ 1               | 6.7 $\pm$ 0.7            | 2.7 $\pm$ 0.3            | 0.90 $\pm$ 0.09          |
| NGC 7213     | 55                 | 4.0 $\pm$ 0.5           |                          | 7.4 $\pm$ 0.8            | 4.7 $\pm$ 0.5            | 1.9 $\pm$ 0.2            | 0.64 $\pm$ 0.07          |
| NGC 7465     | 50                 | 4.4 $\pm$ 0.4           | 6.3 $\pm$ 0.6            | 5.5 $\pm$ 0.6            | 2.5 $\pm$ 0.3            | 1.0 $\pm$ 0.1            | 0.35 $\pm$ 0.05          |
| NGC 7479     | 80                 | 17 $\pm$ 2              | 28 $\pm$ 3               | 29 $\pm$ 3               | 15 $\pm$ 2               | 6 $\pm$ 0.6              | 2.1 $\pm$ 0.2            |
| NGC 7582     | 130                | 70 $\pm$ 7              |                          | 73 $\pm$ 8               | 32 $\pm$ 3               | 13 $\pm$ 1               | 4.0 $\pm$ 0.4            |
