# Supplementary material for: The nuclear and integrated far-infrared emission of nearby Seyfert galaxies
Source: arXiv:1603.04235 ancillary file (2016-03-14)
Supplement: Supplementary file 3 [file galaxies_images.pdf]

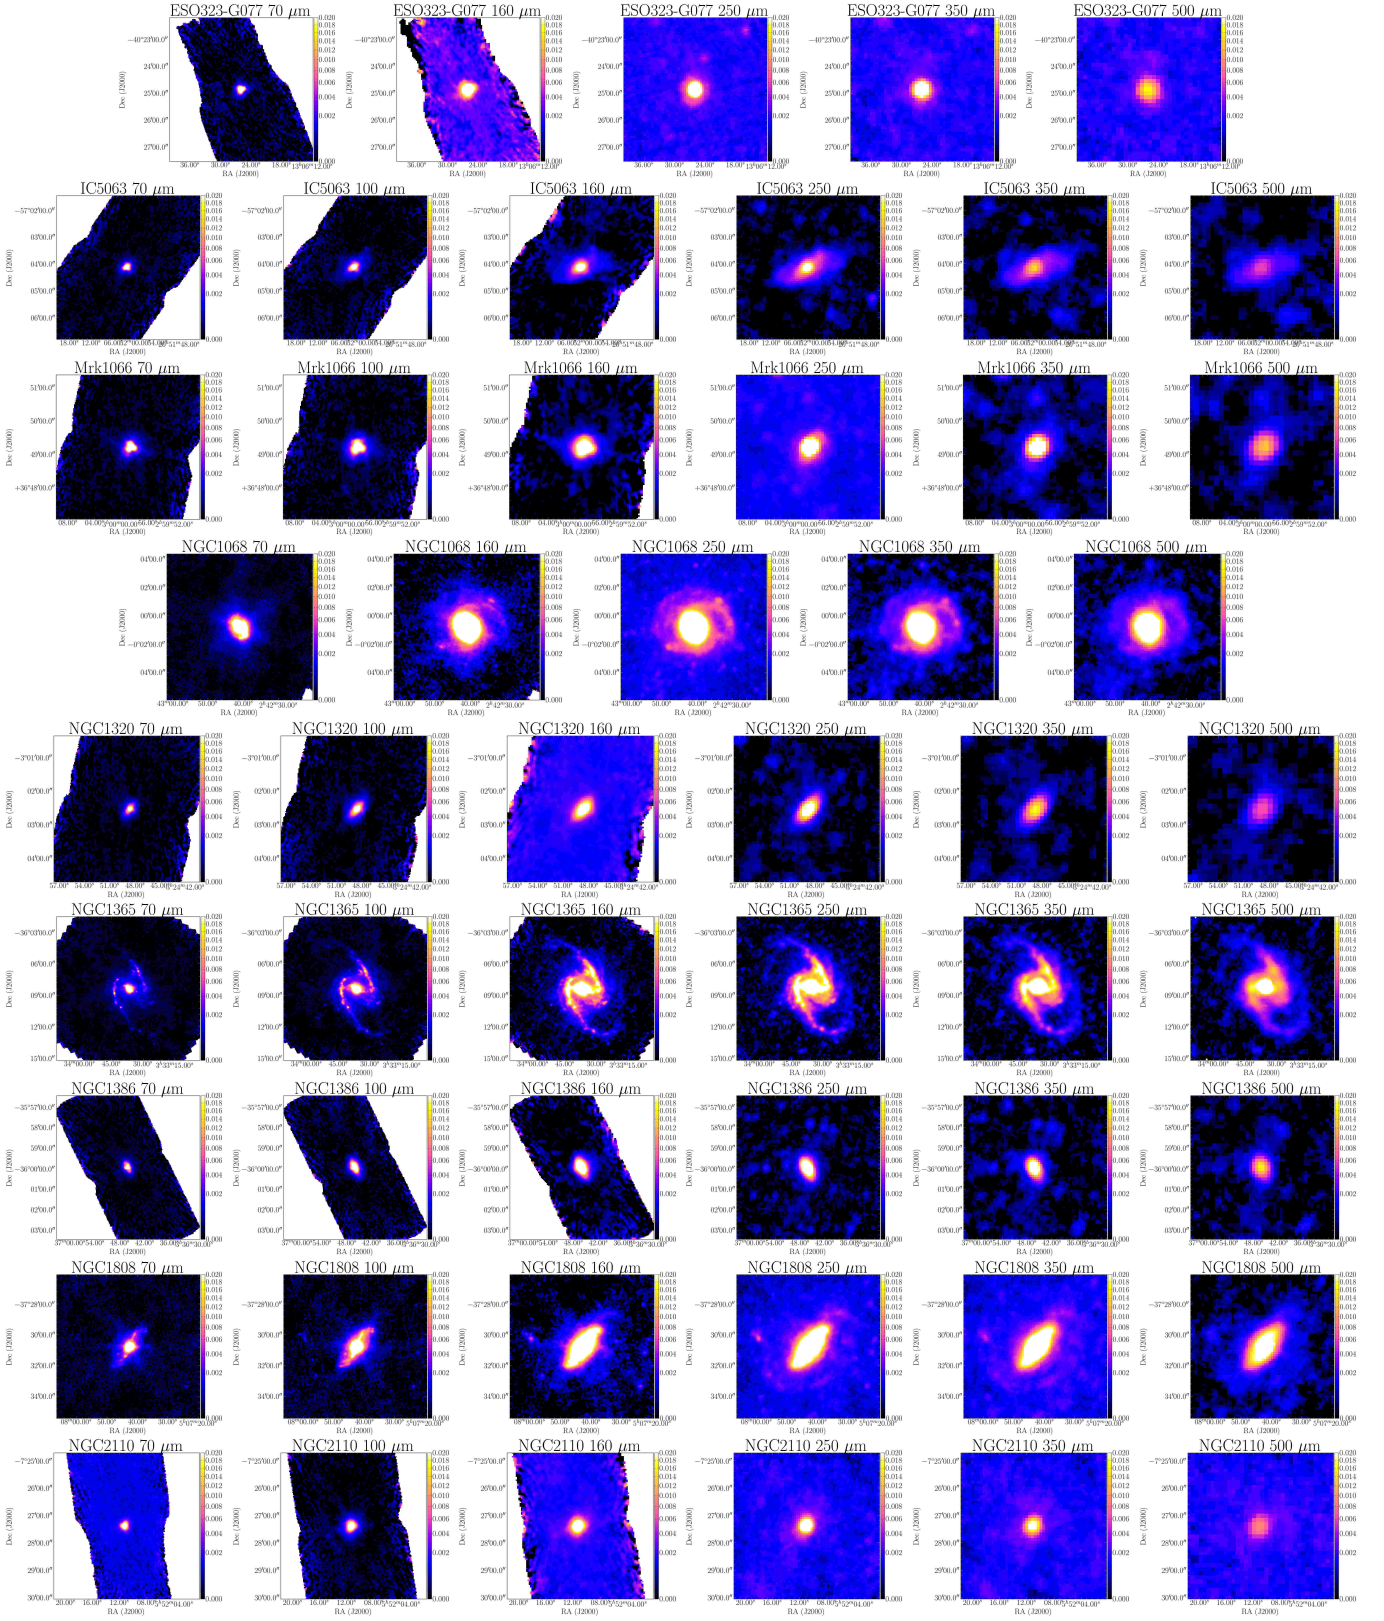

**Figure 1.** Mosaics of the galaxies in the PACS 70, 100, 160 bands (three most left panels, left to right), and in the SPIRE 250, 350, and 500  $\mu\text{m}$  bands (the most right panels from left to right). The images are shown in a square root scale.

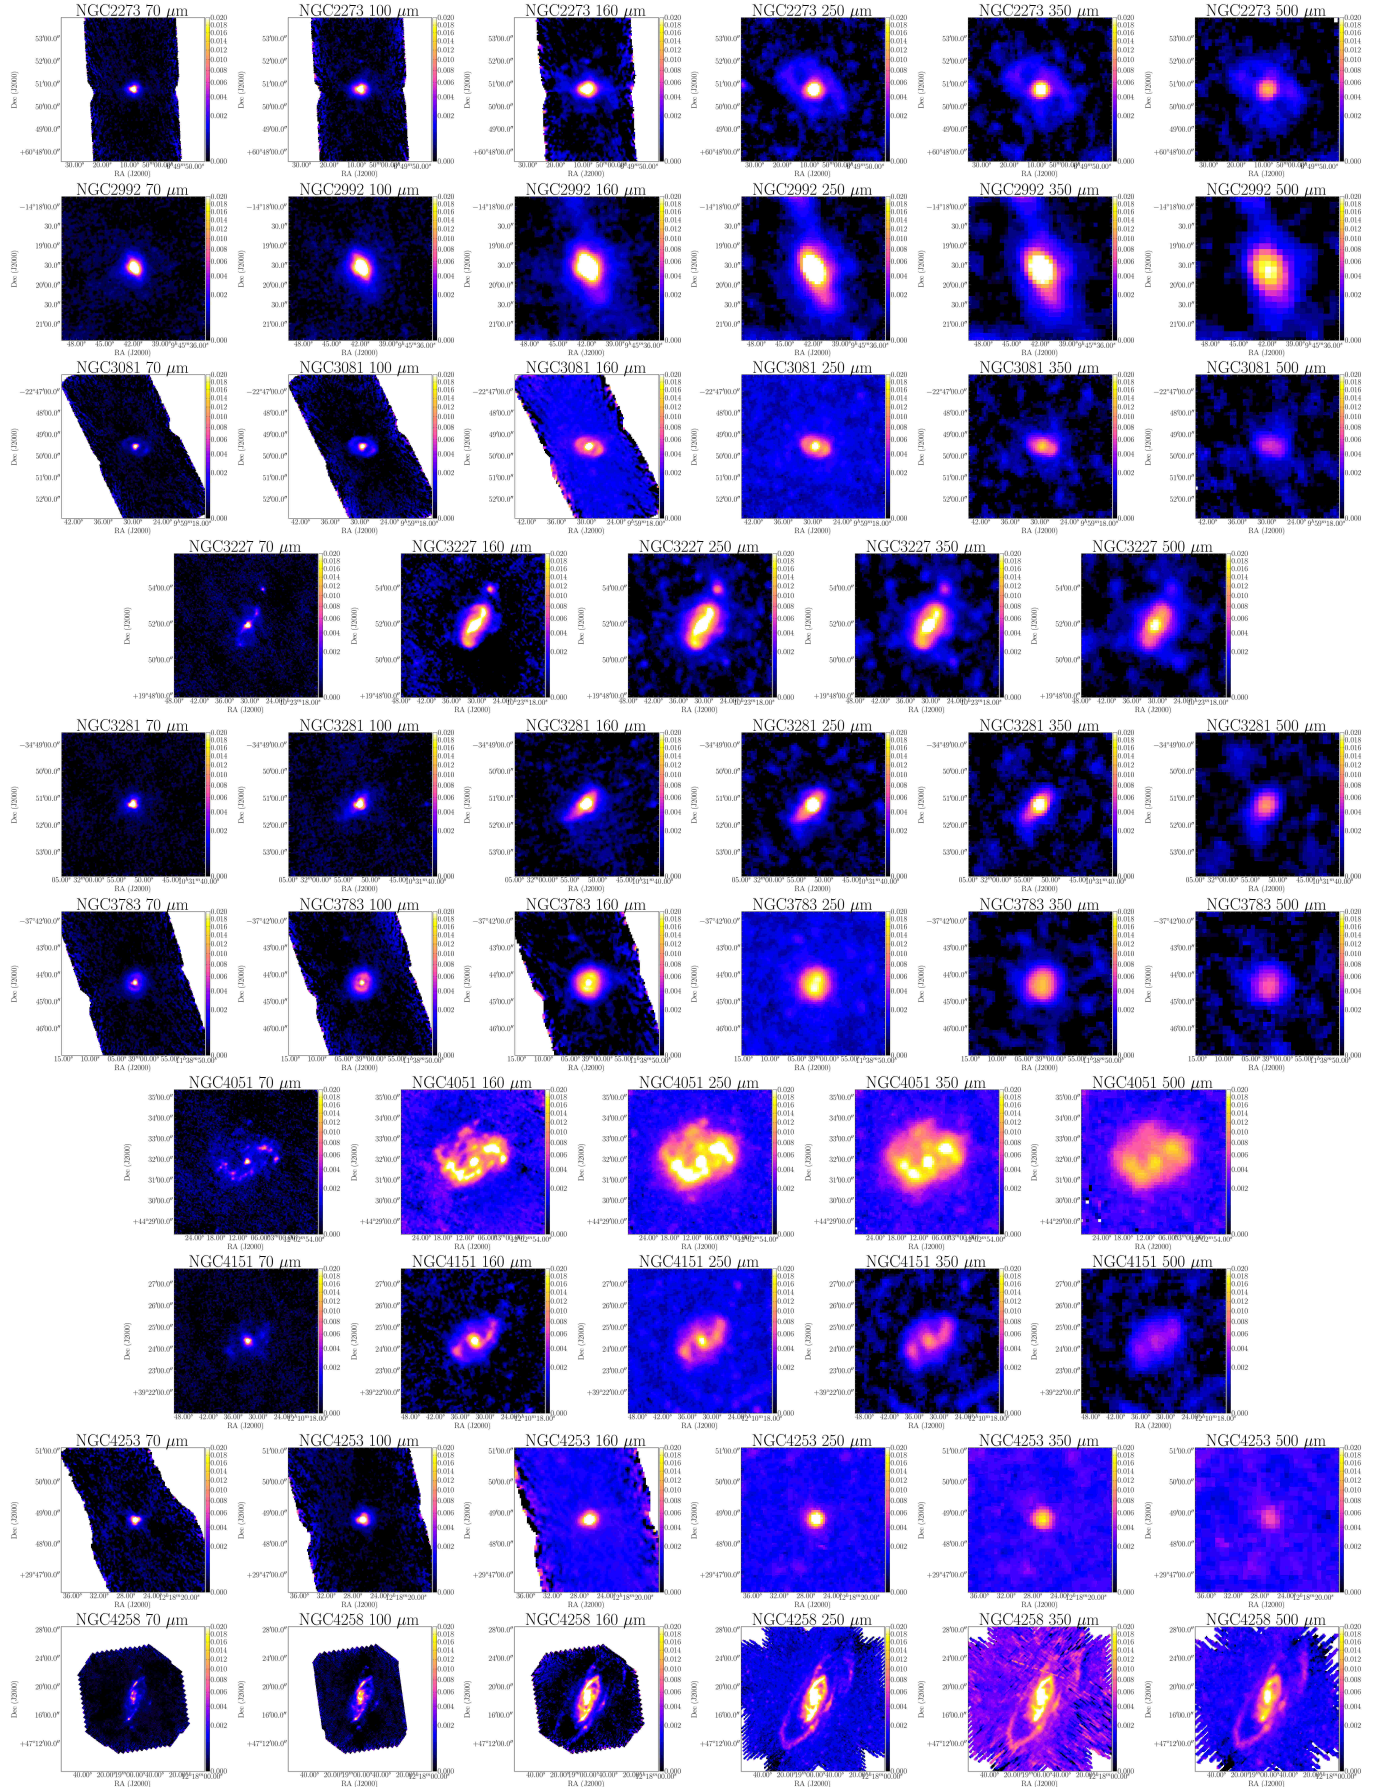

Figure 1 – continued



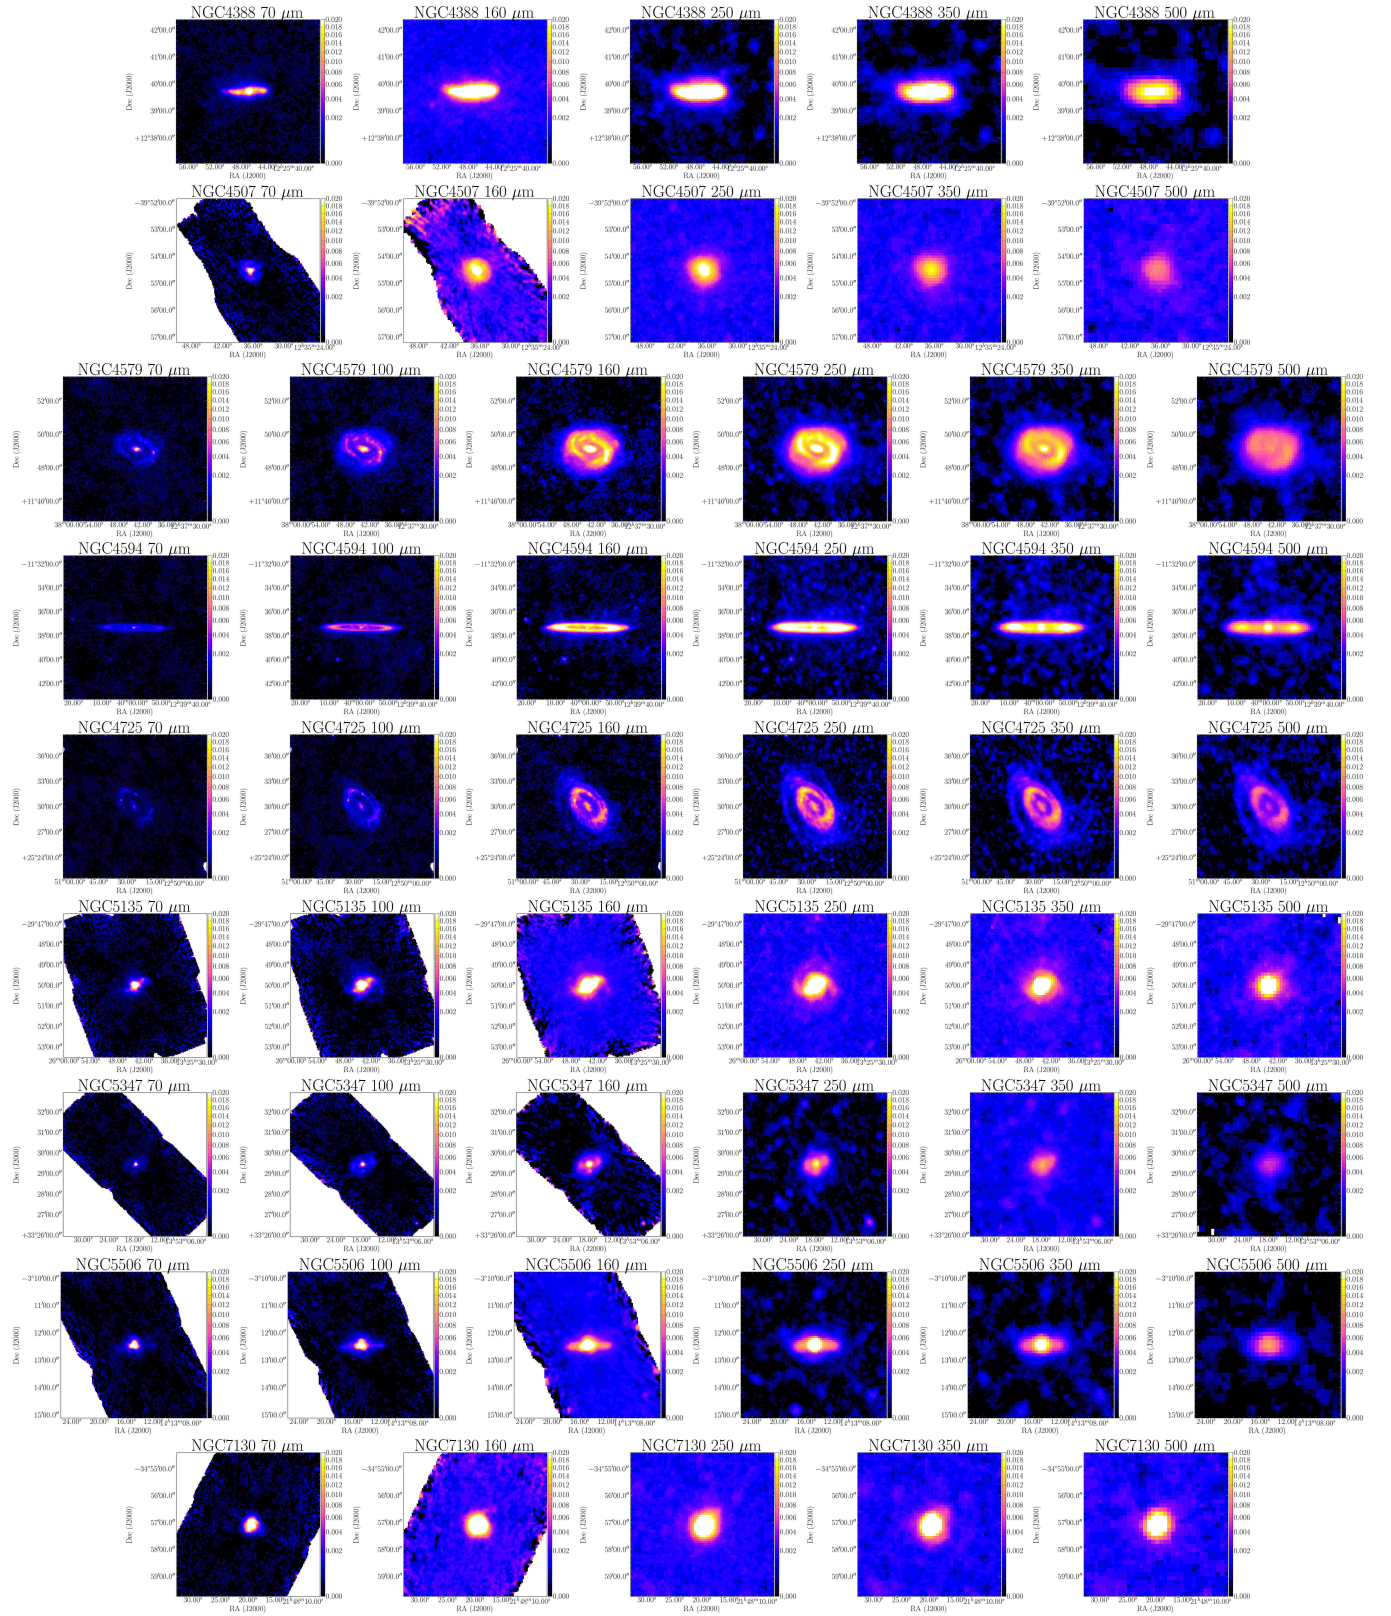

Figure 1 – continued

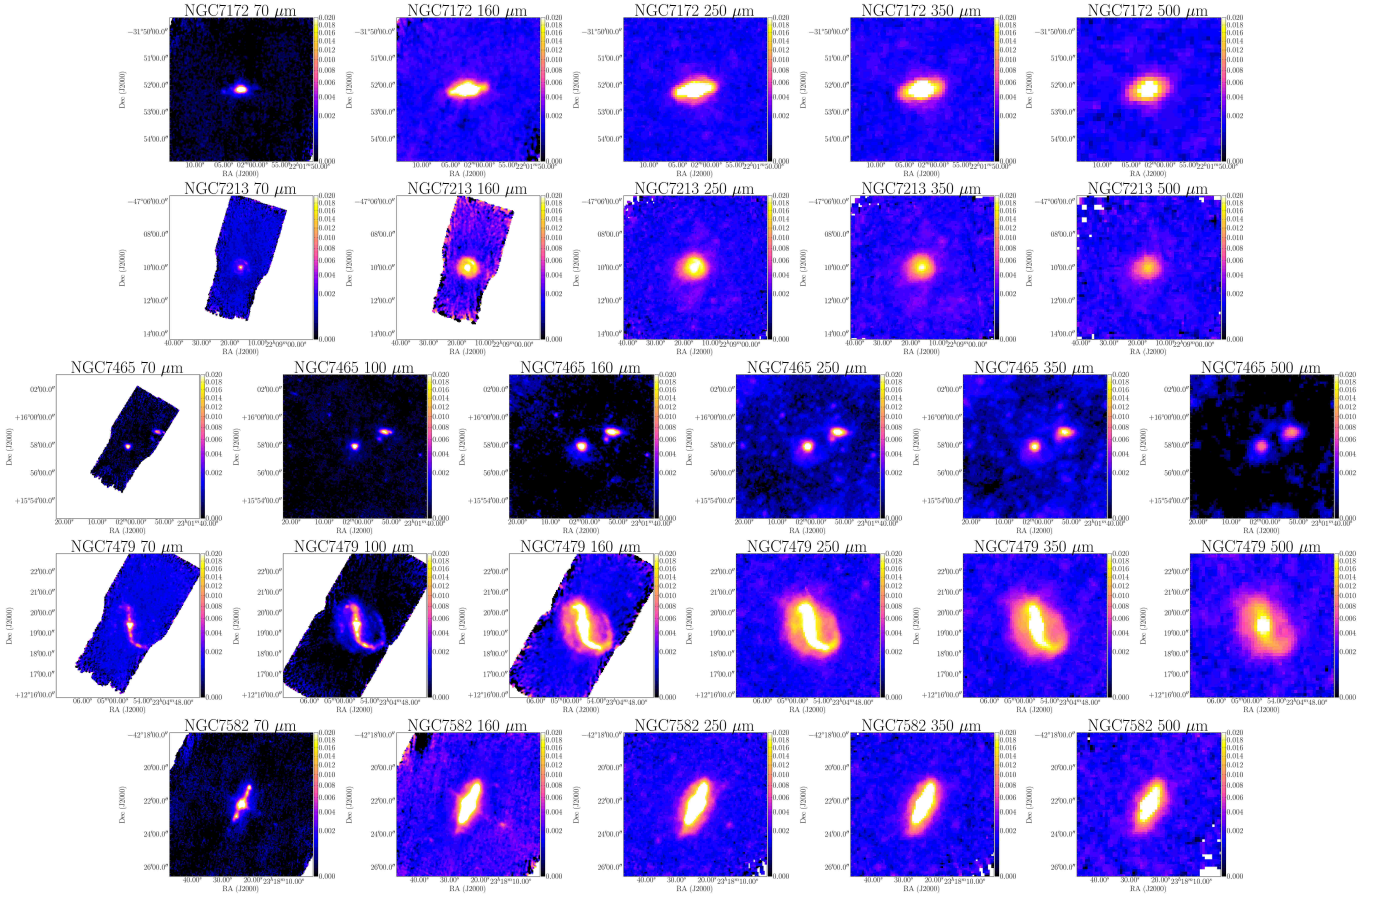Figure 1 – *continued*
