# Supplementary material for: The nuclear and integrated far-infrared emission of nearby Seyfert galaxies
Source: arXiv:1603.04235 ancillary file (2016-03-14)
Supplement: Supplementary file 4 [file integrated_emission_fits_beta=2.pdf]

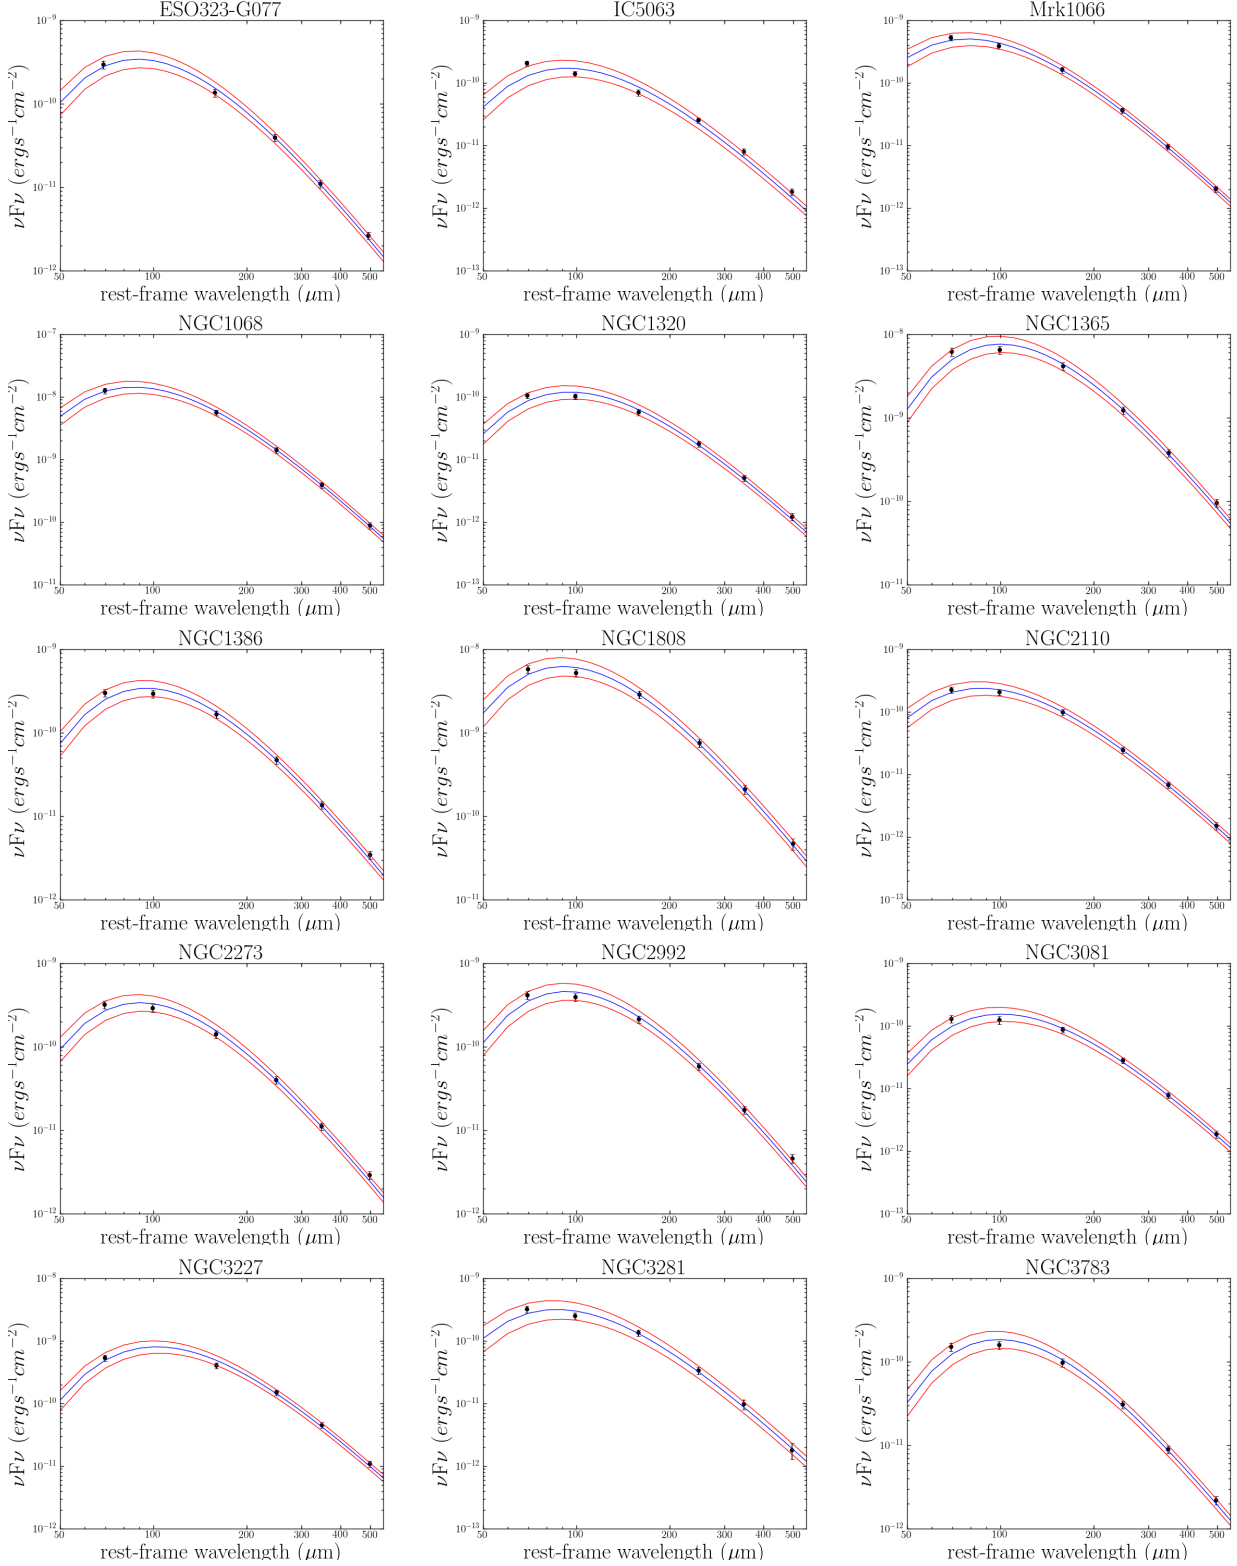

**Figure 1.** Fits to the integrated galaxies SEDs with  $\beta=2$ . The blue line indicates the best fit whereas the red lines delineate the  $\pm 1\sigma$  uncertainty of the best fit.

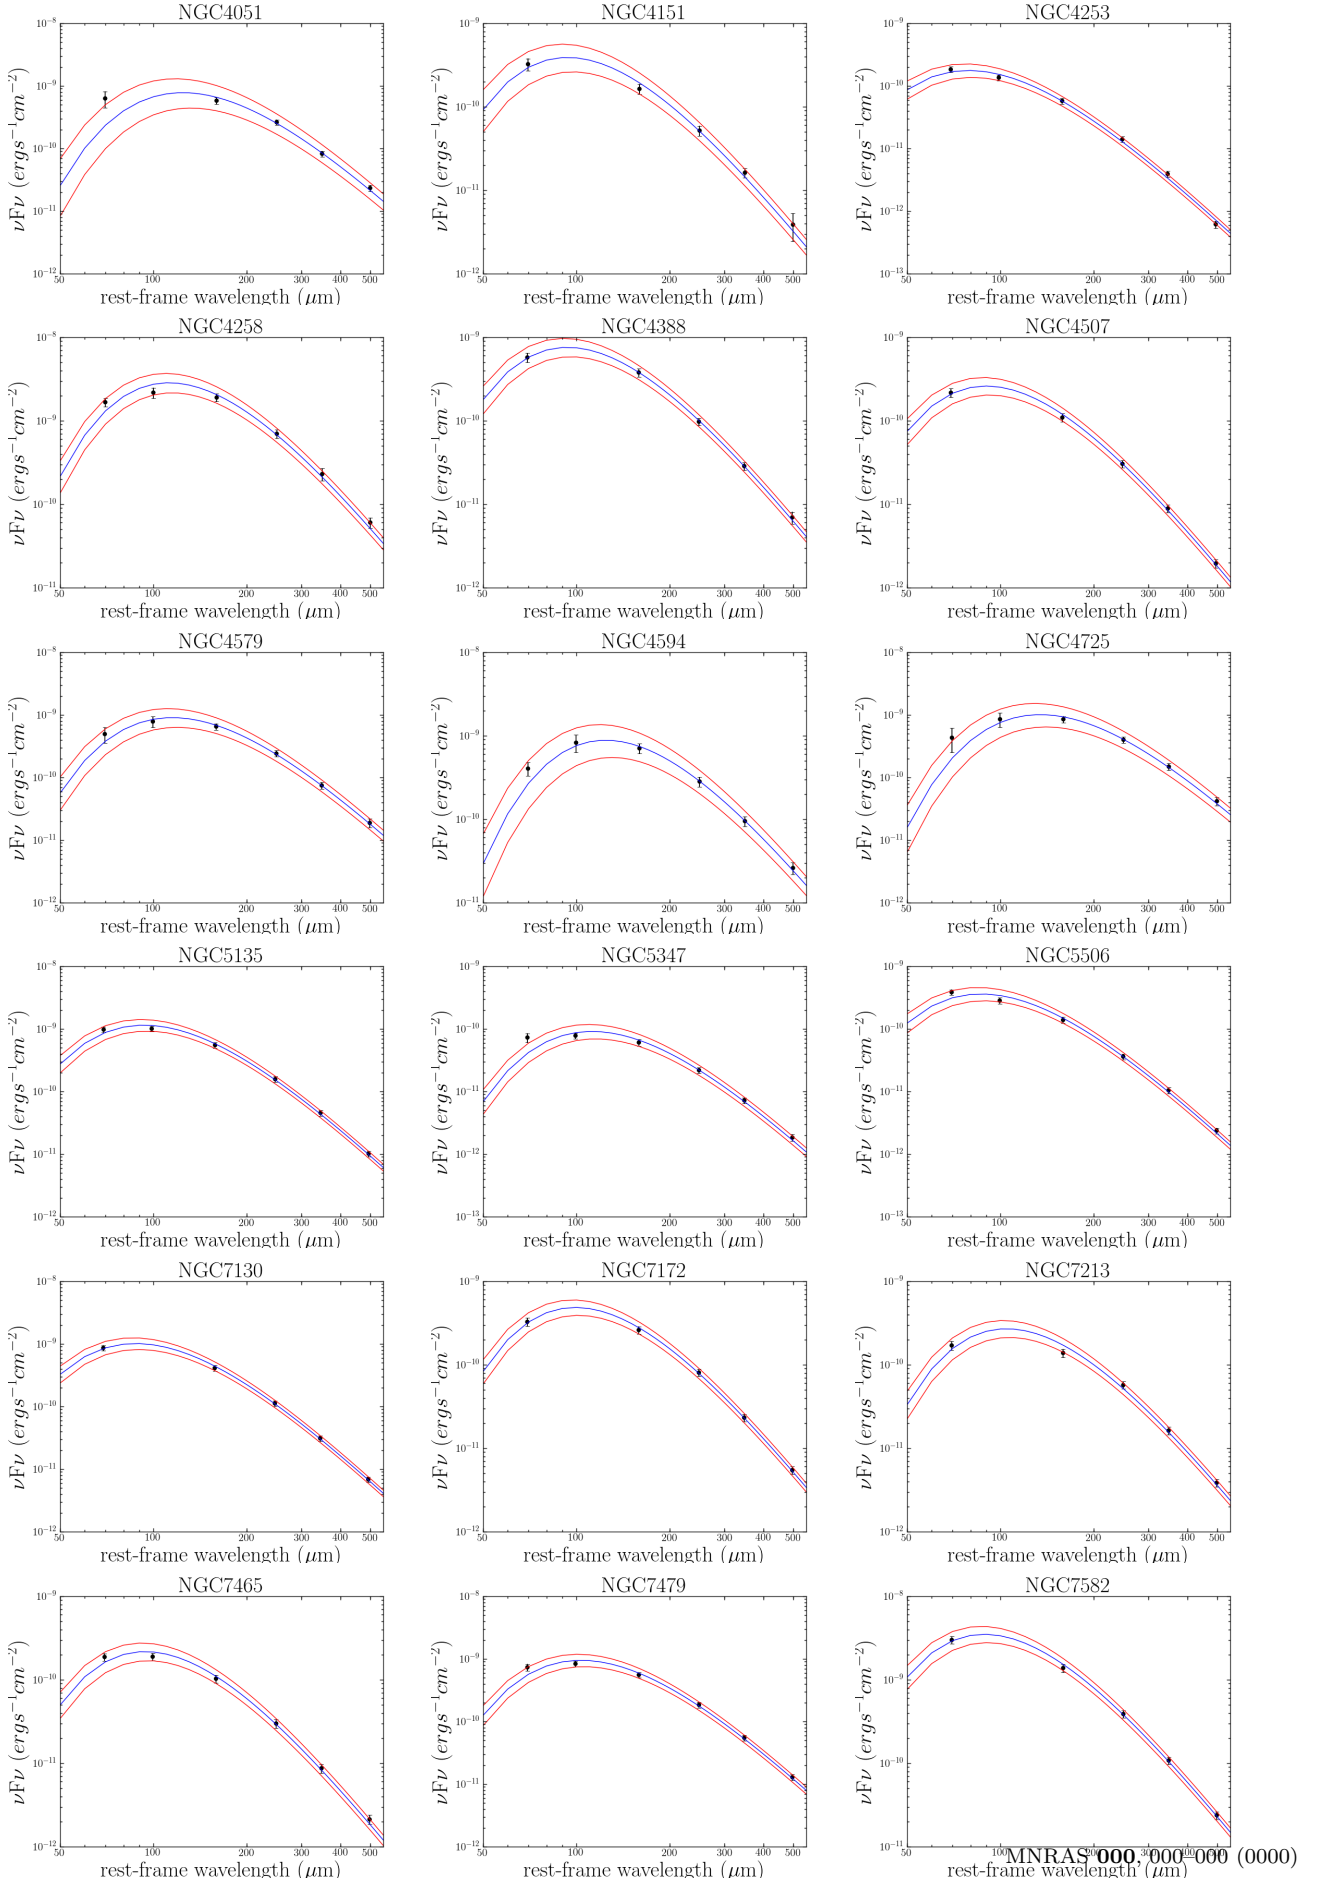

Figure 1 – continued
