# Supplementary material for: The nuclear and integrated far-infrared emission of nearby Seyfert galaxies
Source: arXiv:1603.04235 ancillary file (2016-03-14)
Supplement: Supplementary file 5 [file seds.pdf]

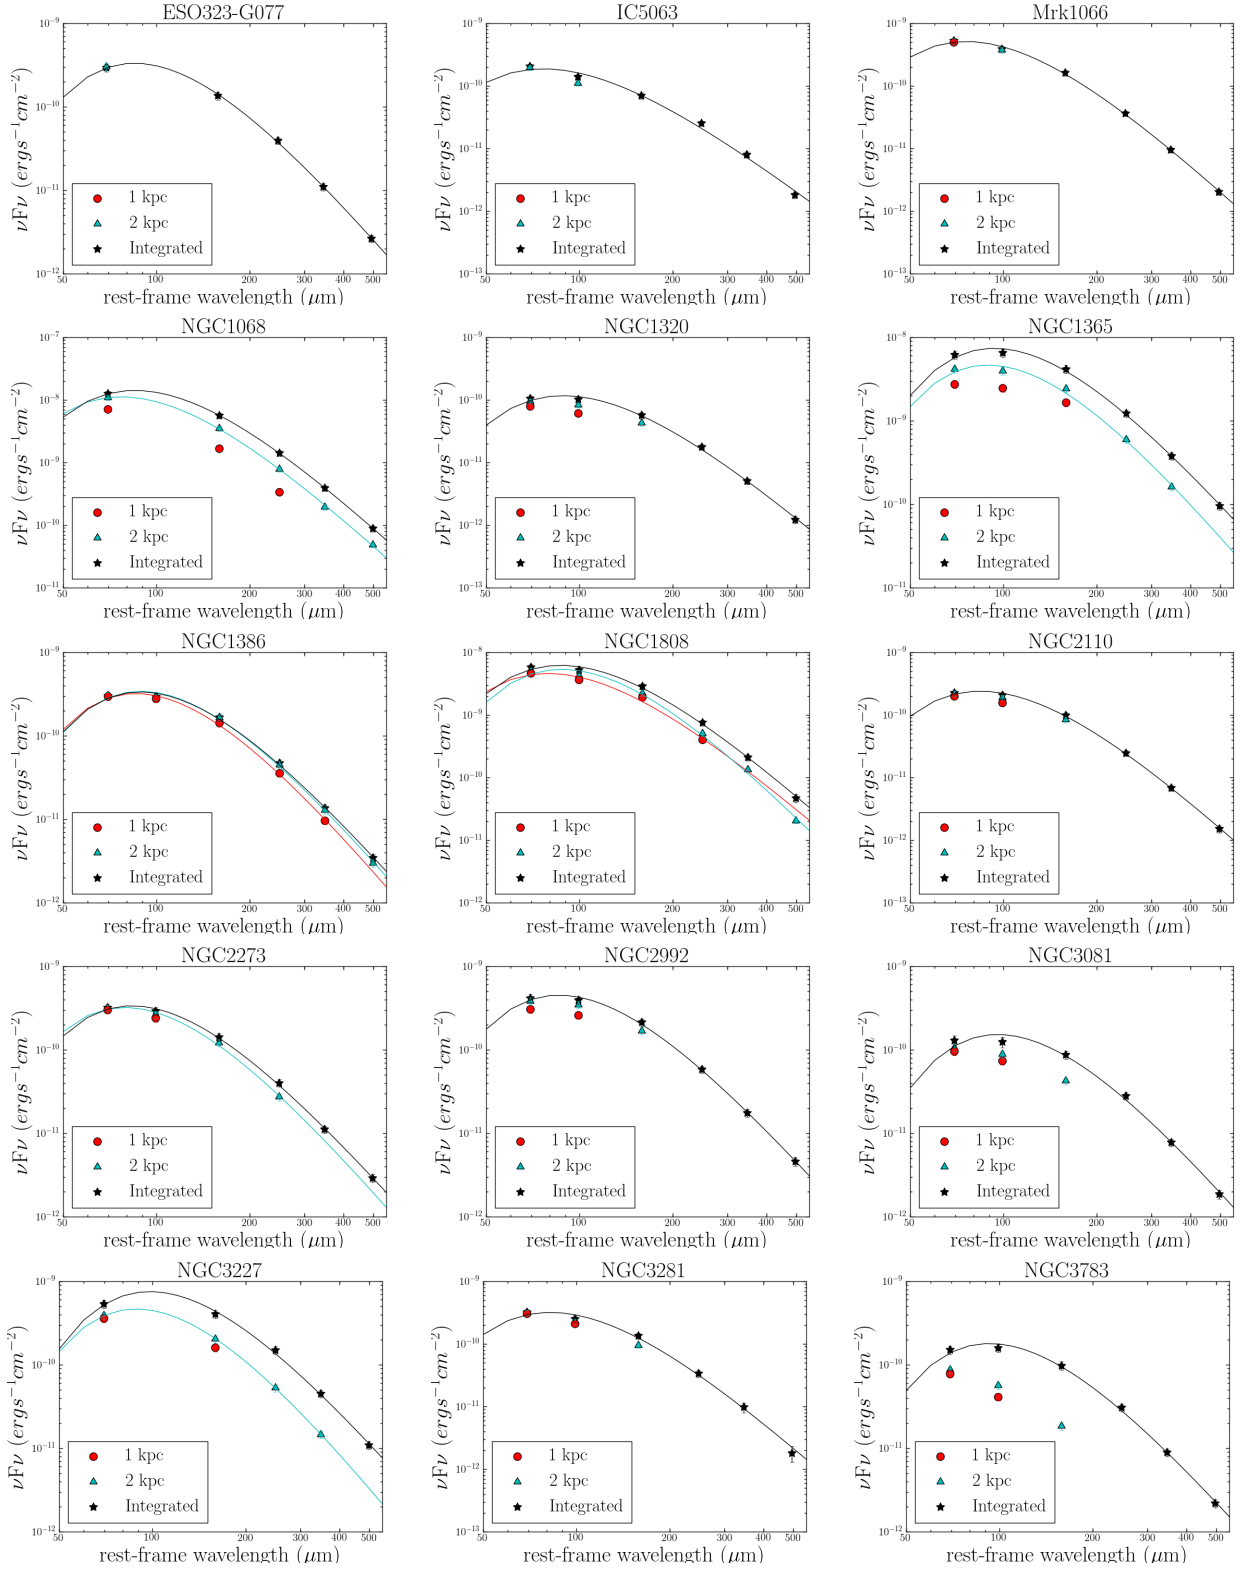

**Figure 1.** Best fits to the FIR SEDs of the galaxies with all the parameters left free to vary. The red circles are the fluxes for  $r = 1$  kpc, the cyan triangles for  $r = 2$  kpc and black stars for the total galaxy. The lines indicate the best fit in each region (only if there are 4 or more data points), with the colours as for the data points.

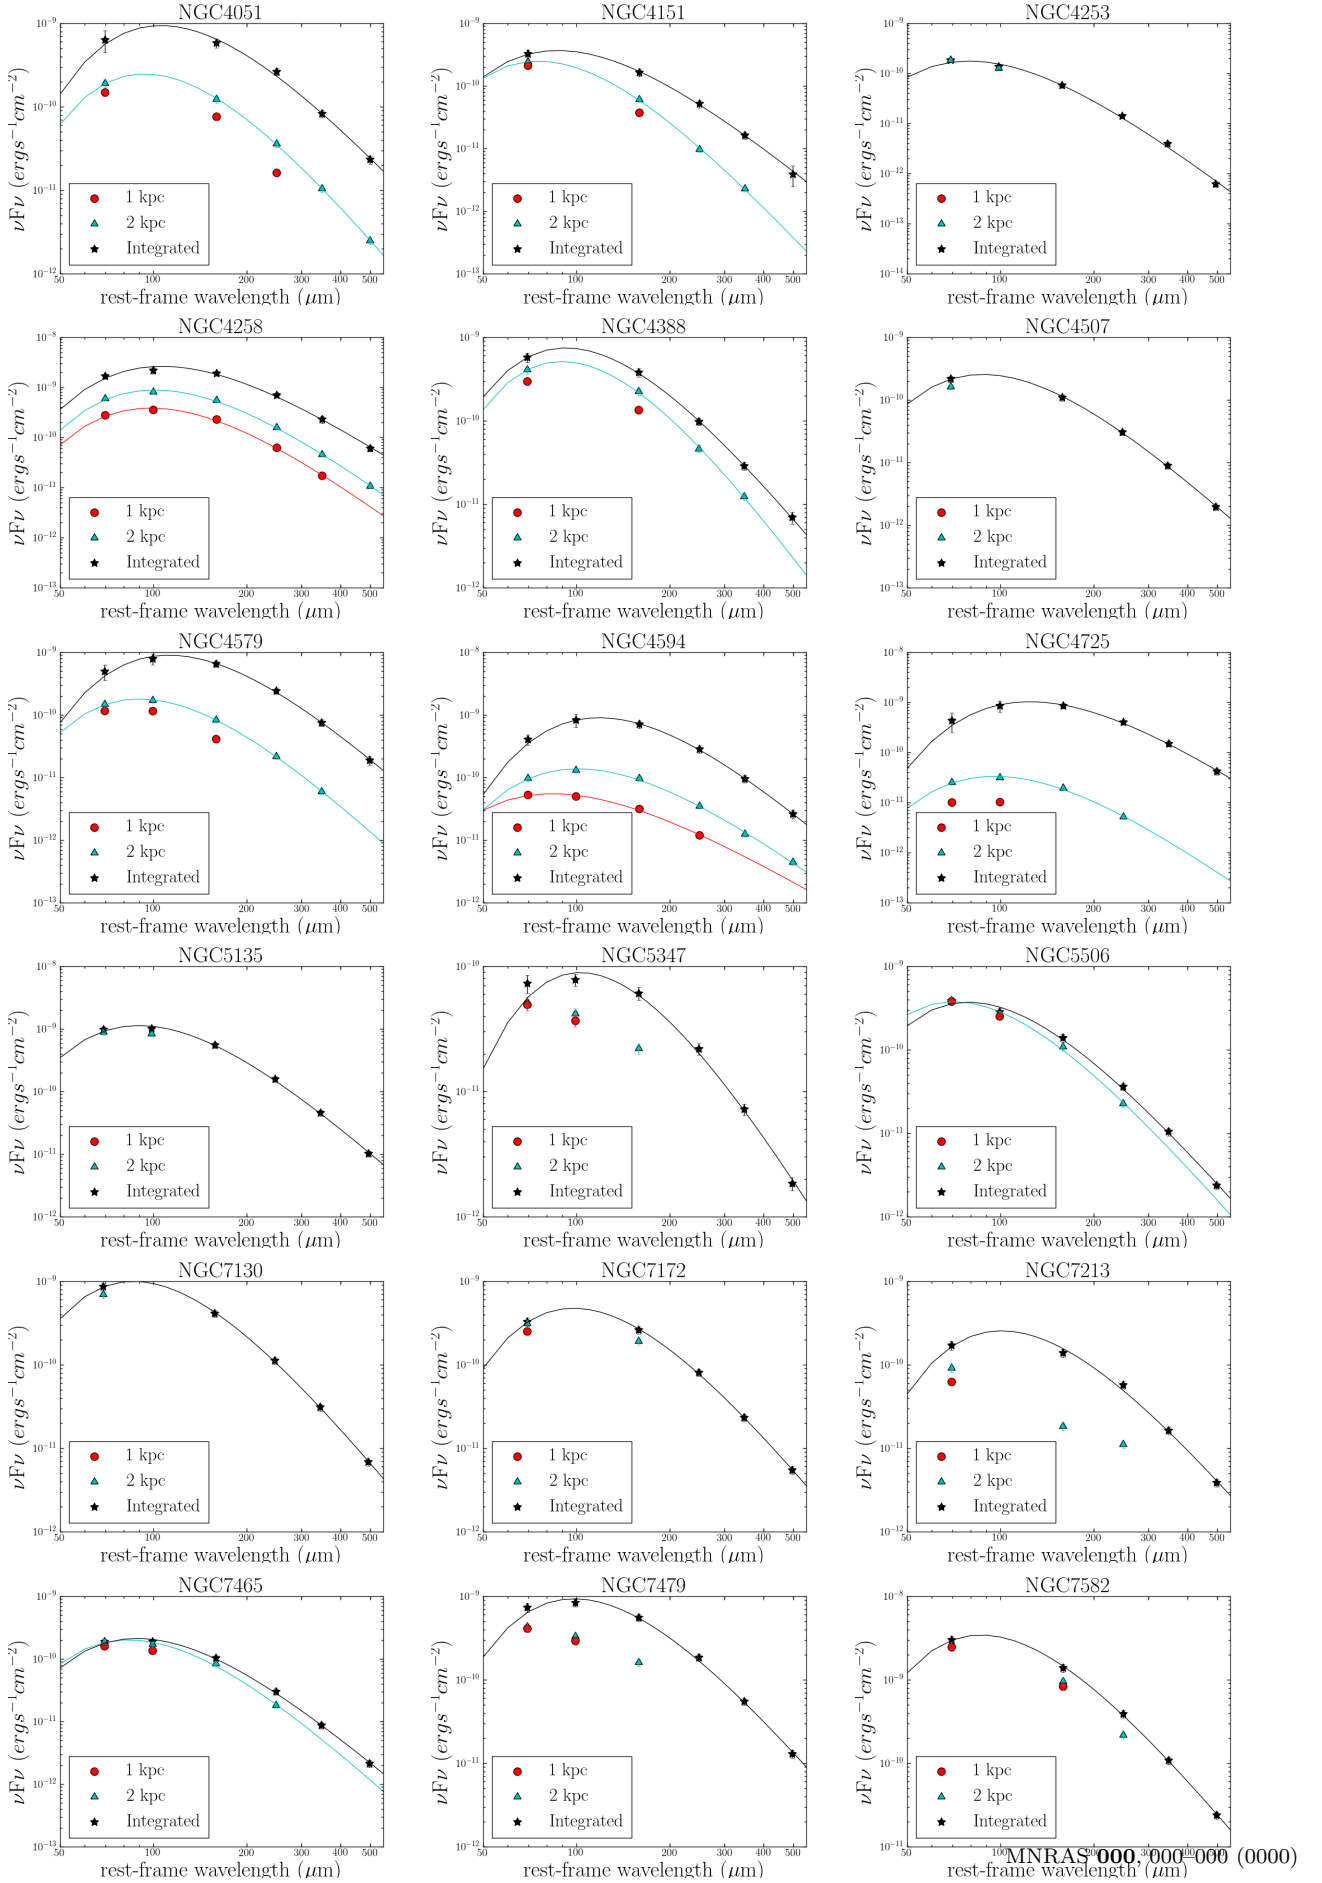

Figure 1 – continued
